# Supplementary material for: Edge: Enriching Knowledge Graph Embeddings with External Text
Source: arXiv:2104.04909 source file (2021-04-11)
Supplement: Supplementary file 1 [file 07-supplement.tex]

In this section, we provide materials to ensure the repeatability of our analysis and reproducibility of our experimental results. We will open source our code upon acceptance of the paper and provide detailed instruction on usage and implementation. 

\subsection{Implementation Details}
Our framework consists of two modules 1) data processing module to generate $a\mathcal{KG}$, and 2) training module to fit two graphs into our deep neural networks architecture.
\subsubsection{data processing Module} As described in subsection \ref{subsec:GT}, generating $a\mathcal{KG}$ involves a multi-step procedure. We present this procedure in Algorithm \ref{alg:gt} one more time to clarify the steps. As this algorithm shows for each target entity in $\mathcal{KG}$, denoted by $e_t$, we perform the following steps:

\begin{algorithm}[ht]
\caption{Construct textual graph $a\mathcal{KG}$}
\begin{algorithmic}[1]
    \Require knowledge graph $\mathcal{KG}$ and external text $\mathcal{T}$.
    \State Initialize $\mathcal{R}_T \leftarrow \{\}$ \label{alg:line:1}
    \For{$e_t$ in $\mathcal{E}_K$} \label{alg:line:2}
        \State $\mathcal{E}_{e_t}\leftarrow$ top $v$ most similar entities to $e_t$. \label{alg:line:3}
        \State $W\leftarrow$ top $w$ keywords of $\mathcal{E}_e$. \label{alg:line:4}
        \State Initialize $S\leftarrow \{\}$
        \For{$k$ in $W$} \label{alg:line:5}
            \State $S =S\ \cup$ wordnet.synsets($k$). \label{alg:line:6}
        \EndFor
        \State $F\leftarrow$ set of $m$ facts extracted from $S$. \label{alg:line:7}
        \For{$t$ in $F$} \label{alg:line:8}
            \State $\mathcal{R}_T$ = $\mathcal{R}_T\cup (t,e)$ \label{alg:line:9}
        \EndFor \label{alg:line:10}
    \EndFor \label{alg:line:11}
    \State $\mathcal{R}_T=\mathcal{R}_K\cup\mathcal{R}_T$ \label{alg:line:12}
    \Ensure $a\mathcal{KG}$ with $\mathcal{R}_T$ as edges 
\end{algorithmic}
\label{alg:gt}
\end{algorithm}

\textbf{Step 1:} Find top $v$ most similar entities to the target entity across all entities of $\mathcal{KG}$. To retrieve semantically similar entities to $e_t$ we use gensim implementation of doc2vec algorithm \cite{mikolov2013efficient} and to retrieve structurally similar entities to $e_t$ we use node2vec library, both in Python. The output of this step is $\mathcal{E}_{e_t}$ (Line \ref{alg:line:3} Algorithm \ref{alg:gt}).

\textbf{Step 2:} Find top keywords across all entities in $\mathcal{E}_{e_t}$. To find these keywords we use gensim implementation of LDA algorithm \cite{blei2003latent} and set the number of topics to 1. By setting the number of topics to 1 we force LDA to find the most expressive keywords around the theme of collection of entities. The output of this step is $W$ (Line \ref{alg:line:4} Algorithm \ref{alg:gt}).

\textbf{Step 3:} Per keyword in $W$ obtain a synset from WordNet. In order to retrieve synsets we use WordNet API that is available in nltk package. The output of this step is $S$ (Line \ref{alg:line:6} Algorithm \ref{alg:gt}).

\textbf{Step 4:} Retrieve facts from $S$. Extracting facts as triplets is different from extracting entities, and fact extraction returns more entities that are not necessarily named entity, hence results in more useful textual features for our task. To extract facts from synsets we use Stanford CoreNLP Jave package. The output of this step is $F$ (Line \ref{alg:line:7} Algorithm \ref{alg:gt}).

\textbf{Step 5:} For every entity, $t_i$, found in $F$ we generate an edge $(t_i,e)$ and add it to the set of edges $\mathcal{R}_T$ (Line \ref{alg:line:9} Algorithm \ref{alg:gt}).

Finally, after populating $\mathcal{R}_T$ for all entities of $\mathcal{KG}$ we take union of $\mathcal{R}_K$ and $\mathcal{R}_T$ and assign it to $\mathcal{R}_T$ (Line \ref{alg:line:12} Algorithm \ref{alg:gt}). See Table \ref{tab:lib} for the list of all libraries used in this study.

\begin{table}[t]
    \centering
    \caption{List of libraries used in this study}
    \resizebox{\columnwidth}{!}{%
    \begin{tabular}{@{}lll@{}} \toprule
        Libraries & Version & Application \\ \midrule \midrule
        Python & & \\ \midrule
        gensim & 3.7.3 & doc2vec and LDA \\
        networkx & 2.3 & graph computation \\
        nltk & 3.4.1 & WordNet API \\
        node2vec & 0.3.0 & node2vec \\
        numpy & 1.15.4 & scientific computing \\
        pymedtermino & 0.3.3 & SNOMED dataset \\
        scikit-learn & 0.21.3 & machine learning models \\
        scipy & 1.3.0 & matrix manipulation \\
        tensorflow & 1.15 or later & deep learning models \\ \midrule \midrule
        Java & & \\ \midrule
        Stanford CoreNLP & 3.9.2 & information extraction \\ \bottomrule
    \end{tabular}
    \label{tab:lib}
    }
\end{table}

\subsubsection{Sensitivity to the choice of components}
Here we replace node2vec with other well known node embedding methods such as DeepWalk and LINE and find similar entities using these algorithms to augment the knowledge graph and show that our model is robust toward the choice of different components of the augmentation process. Table \ref{tab:node_emb} presents AUC and AP performance of the link prediction on Cora dataset for the task of link prediction. We see that the performance is comparable across different methods.

\begin{table}[!ht]
\centering
\caption{Effect of node embedding model for entity selection on final performance.}
\label{tab:node_emb}
\begin{tabular}{@{}lccc@{}}
\toprule
    & DeepWalk & LINE  & node2vec \\ \midrule
AUC & 96.38    & 96.42 & 97.30    \\
AP  & 97.50    & 97.52 & 97.54    \\ \bottomrule
\end{tabular}
\end{table}

\subsubsection{Training Module}
This module is built upon TensorFlow implementation of GAE \cite{kipf2016variational} which provides a two layer GCN architecture. We modify this code so it could fit two graphs at the same time and incorporate our loss function (Equation \ref{eq:loss}) into the optimization process. Here are the list of parameters that we used to obtain the experimental results: 
\begin{itemize}
    \item number of epochs = 200
    \item number of neurons in first GCN layer = 320
    \item number of neurons in second GCN layer = 160
    \item learning rate = 0.001
    \item $\alpha=0.001$, $\beta=10$, $\gamma=1$
    \item optimizer = ADAM
\end{itemize}

\subsection{Datasets}

\subsubsection{Citation Networks}
Cora, Citeseer, and PubMed are three benchmark datasets that are available online publicly. Each node in these graphs represent a paper and it is associated with a text (name or abstract of the paper). In these datasets edges are representative of citations. As we require to generate $a\mathcal{KG}$ we cannot use the preprocessed versions of these datasets that are available online, instead we use our own preprocessing module. The basic statistics of these three datasets are provided in table \ref{tab:data_stat}.

\begin{table}[ht]
    \centering
    \caption{Basic statistics of citation networks}
    \label{tab:data_stat}
    \begin{tabular}{@{}l|cccc@{}} \toprule
        Dataset & \multicolumn{1}{l}{\#nodes} & \multicolumn{1}{l}{\#edges} & \multicolumn{1}{l}{\#classes} & \#features \\ \midrule
        Cora & 2,708 & 5,429 & 7 & 1,433 \\
        Citeseer & 3,312 & 4,732 & 6 & 3,703 \\
        PubMed & 19,717 & 44,338 & 3 & - \\ \bottomrule
    \end{tabular}
\end{table}

\subsubsection{SNOMED Dataset} PyMedTermino is a Python module for easy access to the main medical terminologies in Python including SNOMED. However, the data is not included in the package because of licensing issues. National Library of Medicine (NLM) distributes the SNOMED CT International Edition which is the version we used in our study. After obtaining an academic license the data could be downloaded and used.
